# Supplementary material for: CuLifter: Lifting GPU Binaries to Typed IR
Source: arXiv:2604.27486 source file (2026-09-04)
Supplement: Supplementary file 1 [file appendix.tex]

\section{Pattern Matching Details}
\label{sec:appendix:patterns}
\section{Pattern Matching Details}
\label{sec:appendix:patterns}

This appendix provides the full pattern catalog, matching algorithm, and representative SASS examples for the semantic operation recovery described in Section~\ref{sec:codepattern}.

\subsection{Architecture-Specific Examples}

Listing~\ref{lst:addr-comp-sm52-sm75} shows the same address computation as a three-instruction \texttt{XMAD} chain on SM52 vs.\ a single \texttt{IMAD} on SM75. Listing~\ref{lst:64bit-sub-carry} shows a 64-bit subtraction threading a borrow predicate across \texttt{IADD3}/\texttt{IADD3.X}; handling each instruction alone loses the borrow and produces a wrong result.

\begin{lstlisting}[caption={Architecture-specific address computation.},
                   label={lst:addr-comp-sm52-sm75}]
// sm52: idx = blockIdx.x * blockDim.x + threadIdx.x
XMAD.MRG        R3, R0.reuse, c[0x0][0x8].H1, RZ
XMAD            R2, R0.reuse, c[0x0][0x8], R2
XMAD.PSL.CBCC   R0, R0.H1, R3.H1, R2

// sm75: same computation (single instruction)
IMAD            R6, R6, c[0x0][0x0], R3
\end{lstlisting}

\begin{lstlisting}[caption={64-bit subtraction with carry-threaded IADD3/IADD3.X pattern (SM90).},
                   label={lst:64bit-sub-carry}]
// long long idx = (long long)i - delta
SHF.R.S32.HI  R5,  RZ, 0x1f, R0         // sign-extend i -> {R5, R0}
IADD3    R3, P0, R0, -UR6, RZ            // low:  R3 = R0 - delta_lo; P0 = borrow
IADD3.X  R4, R5, ~UR7, RZ, P0, !PT      // high: R4 = R5 - delta_hi - P0

// idx >= 0 && idx < N  (64-bit range check)
ISETP.GE.U32.AND P0, PT, R3, UR5, PT    // low unsigned:  R3 >=u N_lo?
ISETP.GE.AND.EX  P0, PT, R4, UR4, PT, P0 // high signed+extend: R4 >=s N_hi?
\end{lstlisting}

\subsection{Pattern Matching Algorithm}

\begin{algorithm}
\footnotesize
\caption{Variable-unification-based pattern identification.}
\label{alg:graphmatch}
  \SetKwFunction{PatternMatcher}{PatternMatcher}
  \SetKwFunction{FindSeeds}{FindSeeds}
  \SetKwFunction{MatchOpcodes}{MatchOpcodes}
  \SetKwFunction{Unify}{Unify}

  \PatternMatcher{\textit{BB}, \textit{PatternTable}} { \\
  \KwIn{\textit{BB}: basic block; \textit{PatternTable}: instruction-sequence templates}
  \KwOut{\textit{matches}: matched instruction groups}
    \textit{matches} $\leftarrow$ $\emptyset$ \\
    \For{\textit{pattern} $\in$ \textit{PatternTable}} {
      \textit{seeds} $\leftarrow$ \FindSeeds{\textit{BB}, \textit{pattern.in\_opcodes}} \\
      \For{\textit{candidate} $\in$ \textit{seeds}} {
        \textit{vars} $\leftarrow \emptyset$ \tcp*{variable bindings}
        \textit{ok} $\leftarrow$ \textbf{true} \\
        \For{\textit{(inst, tmpl)} $\in$ \textit{zip(candidate, pattern.templates)}} {
          \If{$\neg$\MatchOpcodes{\textit{inst}, \textit{tmpl}}} {
            \textit{ok} $\leftarrow$ \textbf{false}; \textbf{break}
          }
          \If{$\neg$\Unify{\textit{inst.operands}, \textit{tmpl.vars}, \textit{vars}}} {
            \textit{ok} $\leftarrow$ \textbf{false}; \textbf{break}
          }
        }
        \If{\textit{ok}} {
          \textit{matches} $\leftarrow$ \textit{matches} $\cup$ \{(\textit{pattern.name}, \textit{candidate})\}
        }
      }
    }
    \Return{\textit{matches}}
  }
\end{algorithm}

\subsection{Pattern Catalog}

Table~\ref{tab:specialpatterns} lists all normalization passes and aggregation patterns. Table~\ref{tab:instpatterns} shows representative before/after examples.

\begin{table}[htbp]
\caption{Normalization passes and aggregation patterns implemented in \name{}.}
\begin{center}

\begin{tabular}{l|p{5.2cm}}
\textbf{Pass / Pattern} & \textbf{Description} \\\hline\hline
\multicolumn{2}{l}{\textit{Dedicated normalization passes}} \\\hline
XmadToImad        & Rewrites the 3-instruction SM52 \texttt{XMAD}/\texttt{XMAD.MRG}/\texttt{XMAD.PSL.CBCC} idiom into a single \texttt{IMAD} \\
OpModTransform     & Expands the \texttt{.X4} address-scale modifier by inserting an explicit \texttt{SHL\,2} instruction \\
SRSubstituteReverse & Scans constant-memory operands (\texttt{c[0][offset]}) for known \texttt{SR\_*} offsets (e.g.\ \texttt{SR\_TID.X} at \texttt{0x2C}); inserts explicit \texttt{S2R} instructions at first use and rewrites the operand to the fresh temp register \\
ReciprocalNorm     & Detects the \texttt{I2F}$\to$\texttt{MUFU}$\to$\texttt{IADD}/\texttt{IADD3}$\to$\texttt{F2I} magic-constant reciprocal chain emitted by NVCC; inserts \texttt{BITCAST} nodes around the integer-add step to preserve correct float/int reinterpretation semantics \\\hline
\multicolumn{2}{l}{\textit{Sequence-matching patterns (defined, not yet enabled by default)}} \\\hline
IADD3 + IADD3.X   & 32-bit carry-chain pair $\rightarrow$ 64-bit \texttt{IADD364} \\
ISETP + ISETP.EX  & 64-bit integer compare across two predicate halves $\rightarrow$ \texttt{ISETP64} \\
LEA + LEA.HI.X    & 64-bit effective-address computation $\rightarrow$ \texttt{LEA64} \\
IMAD.WIDE         & Widening 32$\times$32$\rightarrow$64 multiply $\rightarrow$ \texttt{IMAD64} \\
MOV + MOV         & Consecutive 32-bit moves of the same source $\rightarrow$ \texttt{MOV64} \\
SHF (logical)     & \texttt{SHF.R} high-half extraction $\rightarrow$ \texttt{CAST64} or \texttt{SHR64} \\
SHF + SHF / IMAD + SHF & 64-bit left-shift reconstruction $\rightarrow$ \texttt{SHL64} \\
Pack64            & 32-bit register pair $\rightarrow$ 64-bit value via \texttt{PACK64} node \\
\end{tabular}
\label{tab:specialpatterns}
\end{center}
\end{table}

\begin{table}[htbp]
\caption{Representative aggregated instruction patterns.}
\footnotesize
\centering

\begin{tabular}{p{0.55\linewidth}|p{0.38\linewidth}}
\textbf{Instruction pattern (SASS)} & \textbf{Normalized pseudo-instruction} \\ \hline\hline

% XmadToImad: SM52 three-instruction multiply idiom
\footnotesize\verb|XMAD.MRG     R2, R0, R0.H1, RZ|\\
\footnotesize\verb|XMAD         R3, R0, R2, RZ|\\
\footnotesize\verb|XMAD.PSL.CBCC R4, R0.H1, R3, R1|
& \footnotesize\verb|IMAD R4, R0, R0, R1|
\newline \textit{(SM52: three-insn multiply $\rightarrow$ single IMAD)}
\\ \hline

% IADD3/IADD3.X: 64-bit addition carry chain (SM75+)
\footnotesize\verb|IADD3   R1, P1, PT, R2, 0x4, RZ|\\
\footnotesize\verb|IADD3.X R4, RZ,  R6, RZ, P1, PT|
& \footnotesize\verb|IADD364 R4:R1, RZ:R6, 0x4|
\newline \textit{(SM75+: carry-chain pair $\rightarrow$ 64-bit add)}
\\ \hline

% ISETP/ISETP.EX: 64-bit integer comparison
\footnotesize\verb|ISETP.EQ.U32.AND    P0, PT, R6,|\\
\footnotesize\verb|                    0x1, PT|\\
\footnotesize\verb|ISETP.EQ.U32.AND.EX P0, PT, R7,|\\
\footnotesize\verb|                    RZ, PT, P0|
& \footnotesize\verb|ISETP64.EQ.AND P0,|\\
\footnotesize\verb|  R7:R6, 0x1, PT|
\newline \textit{(64-bit compare across two halves)}
\\ \hline

\end{tabular}
\label{tab:instpatterns}
\end{table}

This appendix provides the full pattern catalog, matching algorithm, and representative SASS examples for the semantic operation recovery described in Section~\ref{sec:codepattern}.

\subsection{Architecture-Specific Examples}

Listing~\ref{lst:addr-comp-sm52-sm75} shows the same address computation as a three-instruction \texttt{XMAD} chain on SM52 vs.\ a single \texttt{IMAD} on SM75. Listing~\ref{lst:64bit-sub-carry} shows a 64-bit subtraction threading a borrow predicate across \texttt{IADD3}/\texttt{IADD3.X}; handling each instruction alone loses the borrow and produces a wrong result.

\begin{lstlisting}[caption={Architecture-specific address computation.},
                   label={lst:addr-comp-sm52-sm75}]
// sm52: idx = blockIdx.x * blockDim.x + threadIdx.x
XMAD.MRG        R3, R0.reuse, c[0x0][0x8].H1, RZ
XMAD            R2, R0.reuse, c[0x0][0x8], R2
XMAD.PSL.CBCC   R0, R0.H1, R3.H1, R2

// sm75: same computation (single instruction)
IMAD            R6, R6, c[0x0][0x0], R3
\end{lstlisting}

\begin{lstlisting}[caption={64-bit subtraction with carry-threaded IADD3/IADD3.X pattern (SM90).},
                   label={lst:64bit-sub-carry}]
// long long idx = (long long)i - delta
SHF.R.S32.HI  R5,  RZ, 0x1f, R0         // sign-extend i -> {R5, R0}
IADD3    R3, P0, R0, -UR6, RZ            // low:  R3 = R0 - delta_lo; P0 = borrow
IADD3.X  R4, R5, ~UR7, RZ, P0, !PT      // high: R4 = R5 - delta_hi - P0

// idx >= 0 && idx < N  (64-bit range check)
ISETP.GE.U32.AND P0, PT, R3, UR5, PT    // low unsigned:  R3 >=u N_lo?
ISETP.GE.AND.EX  P0, PT, R4, UR4, PT, P0 // high signed+extend: R4 >=s N_hi?
\end{lstlisting}

\subsection{Pattern Matching Algorithm}

\begin{algorithm}
\footnotesize
\caption{Variable-unification-based pattern identification.}
\label{alg:graphmatch}
  \SetKwFunction{PatternMatcher}{PatternMatcher}
  \SetKwFunction{FindSeeds}{FindSeeds}
  \SetKwFunction{MatchOpcodes}{MatchOpcodes}
  \SetKwFunction{Unify}{Unify}

  \PatternMatcher{\textit{BB}, \textit{PatternTable}} { \\
  \KwIn{\textit{BB}: basic block; \textit{PatternTable}: instruction-sequence templates}
  \KwOut{\textit{matches}: matched instruction groups}
    \textit{matches} $\leftarrow$ $\emptyset$ \\
    \For{\textit{pattern} $\in$ \textit{PatternTable}} {
      \textit{seeds} $\leftarrow$ \FindSeeds{\textit{BB}, \textit{pattern.in\_opcodes}} \\
      \For{\textit{candidate} $\in$ \textit{seeds}} {
        \textit{vars} $\leftarrow \emptyset$ \tcp*{variable bindings}
        \textit{ok} $\leftarrow$ \textbf{true} \\
        \For{\textit{(inst, tmpl)} $\in$ \textit{zip(candidate, pattern.templates)}} {
          \If{$\neg$\MatchOpcodes{\textit{inst}, \textit{tmpl}}} {
            \textit{ok} $\leftarrow$ \textbf{false}; \textbf{break}
          }
          \If{$\neg$\Unify{\textit{inst.operands}, \textit{tmpl.vars}, \textit{vars}}} {
            \textit{ok} $\leftarrow$ \textbf{false}; \textbf{break}
          }
        }
        \If{\textit{ok}} {
          \textit{matches} $\leftarrow$ \textit{matches} $\cup$ \{(\textit{pattern.name}, \textit{candidate})\}
        }
      }
    }
    \Return{\textit{matches}}
  }
\end{algorithm}

\subsection{Pattern Catalog}

Table~\ref{tab:specialpatterns} lists all normalization passes and aggregation patterns. Table~\ref{tab:instpatterns} shows representative before/after examples.

\begin{table}[htbp]
\caption{Normalization passes and aggregation patterns implemented in \name{}.}
\begin{center}

\begin{tabular}{l|p{5.2cm}}
\textbf{Pass / Pattern} & \textbf{Description} \\\hline\hline
\multicolumn{2}{l}{\textit{Dedicated normalization passes}} \\\hline
XmadToImad        & Rewrites the 3-instruction SM52 \texttt{XMAD}/\texttt{XMAD.MRG}/\texttt{XMAD.PSL.CBCC} idiom into a single \texttt{IMAD} \\
OpModTransform     & Expands the \texttt{.X4} address-scale modifier by inserting an explicit \texttt{SHL\,2} instruction \\
SRSubstituteReverse & Scans constant-memory operands (\texttt{c[0][offset]}) for known \texttt{SR\_*} offsets (e.g.\ \texttt{SR\_TID.X} at \texttt{0x2C}); inserts explicit \texttt{S2R} instructions at first use and rewrites the operand to the fresh temp register \\
ReciprocalNorm     & Detects the \texttt{I2F}$\to$\texttt{MUFU}$\to$\texttt{IADD}/\texttt{IADD3}$\to$\texttt{F2I} magic-constant reciprocal chain emitted by NVCC; inserts \texttt{BITCAST} nodes around the integer-add step to preserve correct float/int reinterpretation semantics \\\hline
\multicolumn{2}{l}{\textit{Sequence-matching patterns (defined, not yet enabled by default)}} \\\hline
IADD3 + IADD3.X   & 32-bit carry-chain pair $\rightarrow$ 64-bit \texttt{IADD364} \\
ISETP + ISETP.EX  & 64-bit integer compare across two predicate halves $\rightarrow$ \texttt{ISETP64} \\
LEA + LEA.HI.X    & 64-bit effective-address computation $\rightarrow$ \texttt{LEA64} \\
IMAD.WIDE         & Widening 32$\times$32$\rightarrow$64 multiply $\rightarrow$ \texttt{IMAD64} \\
MOV + MOV         & Consecutive 32-bit moves of the same source $\rightarrow$ \texttt{MOV64} \\
SHF (logical)     & \texttt{SHF.R} high-half extraction $\rightarrow$ \texttt{CAST64} or \texttt{SHR64} \\
SHF + SHF / IMAD + SHF & 64-bit left-shift reconstruction $\rightarrow$ \texttt{SHL64} \\
Pack64            & 32-bit register pair $\rightarrow$ 64-bit value via \texttt{PACK64} node \\
\end{tabular}
\label{tab:specialpatterns}
\end{center}
\end{table}

\begin{table}[htbp]
\caption{Representative aggregated instruction patterns.}
\footnotesize
\centering

\begin{tabular}{p{0.55\linewidth}|p{0.38\linewidth}}
\textbf{Instruction pattern (SASS)} & \textbf{Normalized pseudo-instruction} \\ \hline\hline

% XmadToImad: SM52 three-instruction multiply idiom
\footnotesize\verb|XMAD.MRG     R2, R0, R0.H1, RZ|\\
\footnotesize\verb|XMAD         R3, R0, R2, RZ|\\
\footnotesize\verb|XMAD.PSL.CBCC R4, R0.H1, R3, R1|
& \footnotesize\verb|IMAD R4, R0, R0, R1|
\newline \textit{(SM52: three-insn multiply $\rightarrow$ single IMAD)}
\\ \hline

% IADD3/IADD3.X: 64-bit addition carry chain (SM75+)
\footnotesize\verb|IADD3   R1, P1, PT, R2, 0x4, RZ|\\
\footnotesize\verb|IADD3.X R4, RZ,  R6, RZ, P1, PT|
& \footnotesize\verb|IADD364 R4:R1, RZ:R6, 0x4|
\newline \textit{(SM75+: carry-chain pair $\rightarrow$ 64-bit add)}
\\ \hline

% ISETP/ISETP.EX: 64-bit integer comparison
\footnotesize\verb|ISETP.EQ.U32.AND    P0, PT, R6,|\\
\footnotesize\verb|                    0x1, PT|\\
\footnotesize\verb|ISETP.EQ.U32.AND.EX P0, PT, R7,|\\
\footnotesize\verb|                    RZ, PT, P0|
& \footnotesize\verb|ISETP64.EQ.AND P0,|\\
\footnotesize\verb|  R7:R6, 0x1, PT|
\newline \textit{(64-bit compare across two halves)}
\\ \hline

\end{tabular}
\label{tab:instpatterns}
\end{table}
